# Supplementary material for: Tuning paramagnetic spin-excitations of single adatoms
Source: arXiv:1706.02085 ancillary file (2017-07-10)
Supplement: Supplementary file 1 [file supplementary.pdf]

# Supplemental Material

Julen Ibañez-Azpiroz, Manuel dos Santos Dias,
Benedikt Schweflinghaus, Stefan Blügel, Samir Lounis

(Dated: June 21, 2017)

PACS numbers:

## I. COMPUTATIONAL DETAILS

Density functional theory (DFT) calculations have been performed in the framework of the Korringa-Kohn-Rostoker (KKR) Green function approach, employing the atomic sphere approximation with full charge density[1]. The exchange and correlation effects have been taken into account using the local spin-density approximation (LSDA) as parametrized by Vosko, Wilk and Nusair[2]. The Ag(100) and Cu(111) surfaces were modeled by a slab of 24 layers augmented by two vacuum regions 21.1 Å thick each, using the lattice constants $a = 5.46$ Å and $a = 4.83$ Å, respectively. In the case of MgO/Ag(100), we have considered a slab containing 19 Ag layers plus one MgO layer, as well as intercalated vacuum sites between the Ag atoms. In all systems, we have subsequently constructed a so-called impurity cluster by cutting out a real space region centered around the position to be occupied by the adatom, which is embedded into the substrate. We have employed converged clusters of 43, 55 and 41 sites for the Ag(100), Cu(111) and MgO/Ag(100), respectively. Structural relaxations of the vertical distance of different adatoms where carried out using the QUANTUM-ESPRESSO package[3] by setting the convergence criterion $|F| < 10^{-4}$ Ry a.u.$^{-1}$. In all cases, the distance between adatom and substrate was reduced by approximately 15% with respect to the ideal value. For the sake of comparison, we adopted the same distance for all adatoms. For the time-dependent DFT calculations, the non-magnetic Kohn-Sham (KS) spin-susceptibility was calculated following the approach presented in Refs. 4,5 (see also Supplementary Section III), while the Stoner exchange parameter has been calculated from its definition in terms of the static susceptibilities, $I_s = \chi_{\mathrm{KS}}^{-1}(0) - \chi^{-1}(0)$. Finally, the connection between many body perturbation theory and the TDDFT scheme has been done following the framework presented in Ref. 6.

## II. FURTHER ELECTRONIC PROPERTIES: ADATOMS ON Ag(100) AND MgO/Ag(100)

In Fig. 1 we show the calculated non-magnetic DOS of several *3d, 4d* and *5d* adatoms deposited on Ag(100). The figure shows that the large peaks coming from localized $d$ states acquire a finite width, which ranges from ∼0.2 eV in the case of Cu, up to ∼1 eV in the case of Sc and Y. This feature reveals a strong hybridization of the adatom's $d$ states with

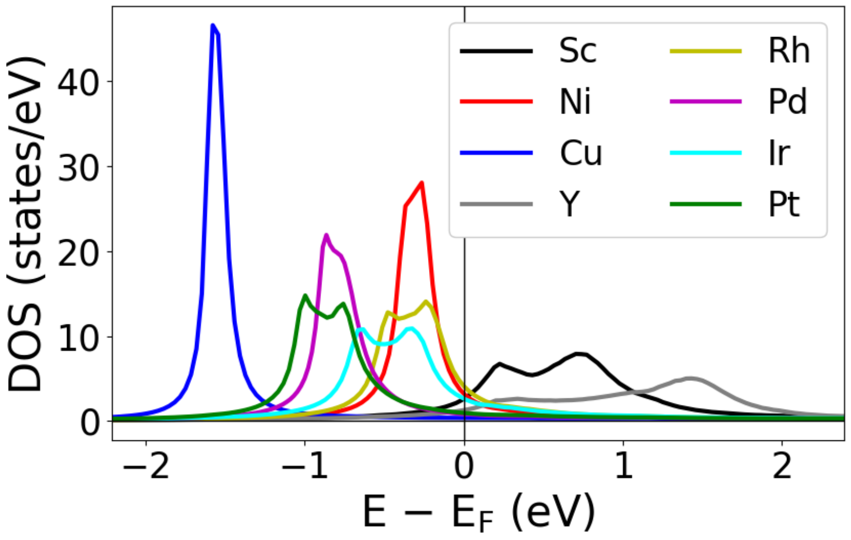


FIG. 1: Calculated non-magnetic DOS of several *3d, 4d* and *5d* adatoms on Ag(100). The vertical line denotes the Fermi level.

| | Sc | Ni | Cu | Y | Rh | Pd | Ir | Pt |
|---|---|---|---|---|---|---|---|---|
| $\rho_F$ (states/eV) | 2.6 | 2.7 | 0.4 | 1.4 | 3.7 | 0.8 | 2.4 | 0.9 |
| $I_s$ (eV) | 0.42 | 0.33 | 0.32 | 0.28 | 0.26 | 0.39 | 0.46 | 0.36 |
| $I_s\rho_F$ | 1.10 | 0.88 | 0.11 | 0.38 | 0.95 | 0.33 | 1.11 | 0.32 |

TABLE I: Calculated values for the DOS at the Fermi level ($\rho_F$), Stoner parameter ($I_s$) and Stoner product ($I_s\rho_F$) for several *3d, 4d* and *5d* adatoms on Ag(100).

the electron bath of the substrate[5,7]. As a consequence, the DOS acquires a finite value at the Fermi level, $\rho_F$, which is listed in Table I for all adatoms, alongside with the calculated Stoner parameter and the resulting Stoner product. We note that the largest $\rho_F$ corresponds to Rh due to the large width of the nearly filled $d$ peak in the DOS and its proximity to the Fermi level (see Fig 1). It is also noteworthy that Sc and Ir, which are predicted to be slightly magnetic, have a smaller $\rho_F$ than Rh and Ni. This is compensated by the Stoner parameter, which is almost 50% larger as compared to Ni and Rh. In this respect, the case of Ni is specially interesting, given that the calculated $I_s$ for the adatom is almost 50% smaller compared to the bulk value[8]. This drop of $I_s$ is the reason why Ni is magnetic in bulk but non-magnetic as an adatom on Ag(100) and other metallic substrates[9,10].

In Fig. 2 we show the calculated non-magnetic DOS for adatoms deposited on

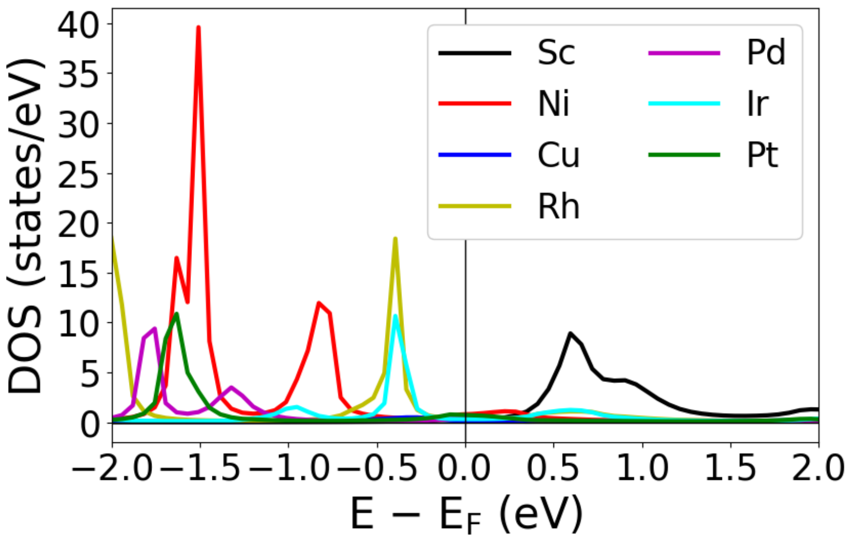


FIG. 2: Calculated non-magnetic DOS of several *3d, 4d* and *5d* adatoms on MgO/Ag(100). The vertical line denotes the Fermi level.

| | Sc | Ni | Cu | Rh | Pd | Ir | Pt |
|---|---|---|---|---|---|---|---|
| $\rho_F$ (states/eV) | 0.2 | 0.8 | 0.2 | 0.4 | 0.6 | 0.4 | 0.8 |
| $I_s$ (eV) | 0.39 | 0.23 | 0.35 | 0.29 | 0.39 | 0.44 | 0.39 |
| $I_s\rho_F$ | 0.09 | 0.18 | 0.06 | 0.12 | 0.25 | 0.19 | 0.30 |

TABLE II: Calculated values for the DOS at the Fermi level ($\rho_F$), Stoner parameter ($I_s$) and Stoner product ($I_s\rho_F$) for several *3d, 4d* and *5d* adatoms on MgO/Ag(100).

MgO/Ag(100). Contrary to Ag(100), this substrate is insulating due to the MgO layer. In overall, this results in a much weaker hybridization of the electrons, which translates into a sharper width of the DOS peaks, as clearly inferred from the comparison between Figs. 2 and 1. In practice, this leads to a much smaller contribution of the DOS at the Fermi level, as summarized in Table II. Given that the calculated Stoner parameter does not vary substantially depending on the substrate, the Stoner product of these non-magnetic elements on MgO/Ag(100) is much smaller than in metallic substrates (compare data in Tables I and II).

## III. AB-INITIO CALCULATION OF THE LONGITUDINAL KOHN-SHAM SPIN-SUSCEPTIBILITY

In this section we provide the ab-initio expression used for the calculation of the longitudinal Kohn-Sham spin-susceptibility. The derivation follows that of Ref. 5, which was done for the transverse component. The considered Hamiltonian of the non-interacting Kohn-Sham system is

$$H^{KS} = \sigma_0 H_0^{KS} + \sigma_z (B^{xc} + B^{ext}), \tag{1}$$

with $H_0^{KS} = T + V^H$. Here, $\sigma_0$ and $\sigma_z$ are respectively the $2 \times 2$ identity and $z$ Pauli spin matrices, $T$ is the electron kinetic energy, and $V^H$, $B^{xc}$ and $B^{ext}$ are the Hartree, exchange-correlation and external potentials, respectively.

We will consider single particle Green's functions (GFs), formally defined as

$$G(E) = (E - H^{KS})^{-1}. \tag{2}$$

In the real-space representation the GFs are written as

$$G(\vec{r}, \vec{r}\,'; E) = \sum_n \frac{\langle \vec{r}|n\rangle \langle n|\vec{r}\,'\rangle}{E - E_n}, \tag{3}$$

where $E$ is a complex energy and $|n\rangle$ are basis functions with eigenvalues $E_n$. We distinguish between retarded and advanced single particle GFs, $G^+(E+i0)$ and $G^-(E-i0)$ respectively, which fulfill

$$\begin{aligned} \mathrm{Re}\, G(E) &= \frac{G^+(E+i0) + G^-(E-i0)}{2}, \\ \mathrm{Im}\, G(E) &= \frac{G^+(E+i0) - G^-(E-i0)}{2i}. \end{aligned} \tag{4}$$

Note that the GFs are $2 \times 2$ diagonal spin matrices, *i.e.*,

$$G \equiv \begin{pmatrix} G^{\uparrow} & 0 \\ 0 & G^{\downarrow} \end{pmatrix}. \tag{5}$$

The general expression for the non-interacting longitudinal spin-susceptibility for a single adatom in terms of GFs is given by[5]

$$\begin{aligned} \chi^{KS}(\vec{r}, \vec{r}\,'; \omega) = -\frac{1}{\pi} \int dE f(E) \mathrm{Tr}\Big[ & \mathrm{Im}[G(\vec{r}, \vec{r}\,'; E)] \sigma_z G^+(\vec{r}\,', \vec{r}; E + \omega + i0) \sigma_z \\ & + \mathrm{Im}[G(\vec{r}\,', \vec{r}; E)] \sigma_z G^-(\vec{r}, \vec{r}\,'; E - \omega - i0) \sigma_z \Big], \end{aligned} \tag{6}$$

with $\sigma_z$ the Pauli spin matrix and $f(E)$ the Fermi-Dirac distribution function. Inserting all quantities in spin-matrix form in Eq. 6, using Eq. 4 to substitute $G^+(E+i0)$ and $G^-(E-i0)$, and taking the trace in the zero temperature limit one obtains

$$\chi^{KS}(\vec{r},\vec{r}\,';\omega) = \sum_\sigma \frac{i}{2\pi}\int_{-\infty}^{E_F} dE\big(G^\sigma(\vec{r},\vec{r}\,';E)G^\sigma(\vec{r}\,',\vec{r};E+\omega) - G^{*\sigma}(\vec{r},\vec{r}\,';E)G^\sigma(\vec{r}\,',\vec{r};E+\omega) + G^\sigma(\vec{r}\,',\vec{r};E)G^{*\sigma}(\vec{r},\vec{r}\,';E-\omega) - G^{*\sigma}(\vec{r}\,',\vec{r};E)G^{*\sigma}(\vec{r},\vec{r}\,';E-\omega)\big). \tag{7}$$

The above shows a convolution between two GFs. Following Ref. 5, the KS spin-susceptibility can be separated into an analytic and non-analytic term denoted respectively by $I_1$ and $I_2$:

$$I_1(\vec{r},\vec{r}\,';\omega) = \sum_\sigma \frac{i}{2\pi}\int_{-\infty}^{E_F} dE\big(G^\sigma(\vec{r},\vec{r}\,';E)G^\sigma(\vec{r}\,',\vec{r};E+\omega) - G^{*\sigma}(\vec{r}\,',\vec{r};E)G^{*\sigma}(\vec{r},\vec{r}\,';E-\omega)\big) \tag{8}$$

$$I_2(\vec{r},\vec{r}\,';\omega) = \sum_\sigma \frac{i}{2\pi}\int_{-\infty}^{E_F} dE\big(G^\sigma(\vec{r}\,',\vec{r};E)G^{*\sigma}(\vec{r},\vec{r}\,';E-\omega) - G^{*\sigma}(\vec{r},\vec{r}\,';E)G^\sigma(\vec{r}\,',\vec{r};E+\omega)\big) \tag{9}$$

Given that $\omega$ is small as compared to $E_F$, it is computationally efficient to rearrange the above two terms. For this, we perform a change of variables $E \rightarrow E-\omega$ in the second terms of both Eqs. 8 and 9, getting

$$I_1(\vec{r},\vec{r}\,';\omega) = \sum_\sigma \frac{i}{2\pi}\int_{-\infty}^{E_F-\omega} dE\big(G^\sigma(\vec{r},\vec{r}\,';E)G^\sigma(\vec{r}\,',\vec{r};E+\omega) - G^{*\sigma}(\vec{r}\,',\vec{r};E)G^{*\sigma}(\vec{r},\vec{r}\,';E+\omega)\big) + \sum_\sigma \frac{i}{2\pi}\int_{E_F-\omega}^{E_F} dE G^\sigma(\vec{r},\vec{r}\,';E)G^\sigma(\vec{r}\,',\vec{r};E+\omega) \tag{10}$$

$$I_2(\vec{r},\vec{r}\,';\omega) = -\sum_\sigma \frac{i}{2\pi}\int_{E_F-\omega}^{E_F} dE G^{*\sigma}(\vec{r},\vec{r}\,';E)G^\sigma(\vec{r}\,',\vec{r};E+\omega). \tag{11}$$

Then, adding the last term of Eq. 10 to Eq. 11, we obtain the expressions used for our calculations:

$$\bar{I}_1(\vec{r},\vec{r}\,';\omega) = \sum_\sigma \frac{i}{2\pi}\int_{-\infty}^{E_F-\omega} dE\big(G^\sigma(\vec{r},\vec{r}\,';E)G^\sigma(\vec{r}\,',\vec{r};E+\omega) - G^{*\sigma}(\vec{r}\,',\vec{r};E)G^{*\sigma}(\vec{r},\vec{r}\,';E+\omega)\big) \tag{12}$$

$$\bar{I}_2(\vec{r},\vec{r}\,';\omega) = \sum_\sigma \frac{i}{2\pi}\int_{E_F-\omega}^{E_F} dE G^\sigma(\vec{r},\vec{r}\,';E+\omega)\big(G^\sigma(\vec{r}\,',\vec{r};E) - G^{*\sigma}(\vec{r},\vec{r}\,';E)\big) \tag{13}$$

$\bar{I}_1$ is analytic because it involves GFs that are analytic in the same half complex plane, therefore it can be efficiently calculated using a regular contour mesh [11] with modest computational effort. $\bar{I}_2$ is non-analytic and thus must be calculated along a line parallel to the real axis, which is usually computationally very heavy. However, since we managed to set the integration range of Eq. 13 to a small energy window controlled by $\omega$, the calculations can then be readily carried out.

## IV. FREQUENCY EXPANSION OF THE LONGITUDINAL SPIN-SUSCEPTIBILITY

The frequency expansion of the longitudinal spin-susceptibility discussed in the main text is

$$\chi^{KS}(\omega) = \chi^{KS}(0) + i\alpha\omega + \mathcal{O}(\omega^2), \tag{14}$$

with $\alpha \equiv \mathrm{Im}\, \partial\chi^0(\omega)/\partial\omega\Big|_{\omega=0}$. Note that $\chi^{KS}(\omega)$ in the above equation is an adatom-averaged quantity of the spatially dependent spin-susceptibility $\chi^{KS}(\vec{r},\vec{r}\,';\omega)$,

$$\chi^{KS}(\omega) = \int d\vec{r} \int d\vec{r}\,'\chi^{KS}(\vec{r},\vec{r}\,';\omega). \tag{15}$$

For the calculations that will follow, it will be useful to consider the following identities of the single-particle GFs defined in Eq. 3 (see, *e.g.*, Ref. 7):

$$G(\vec{r},\vec{r}\,';E\pm\omega) = G(\vec{r},\vec{r}\,';E) \mp \int d\vec{r}_1 G(\vec{r},\vec{r}_1;E)\omega G(\vec{r}_1,\vec{r}\,';E\pm\omega), \tag{16}$$

$$\lim_{\omega\to 0} G(\vec{r},\vec{r}\,';E\pm\omega) \simeq G(\vec{r},\vec{r}\,';E) \mp \int d\vec{r}_1 G(\vec{r},\vec{r}_1;E)\omega G(\vec{r}_1,\vec{r}\,';E), \tag{17}$$

$$\frac{\partial G(\vec{r},\vec{r}\,';E\pm\omega)}{\partial\omega}\Big|_{\omega=0} \simeq \mp \int d\vec{r}_1 G(\vec{r},\vec{r}_1;E)G(\vec{r}_1,\vec{r}\,';E) = \pm\frac{\partial G(\vec{r},\vec{r}\,';E)}{\partial E}. \tag{18}$$

Eq. 17 can be checked by direct insertion of the definition of the GFs, Eq. 3, into the right hand side. The approximate equality in Eq. 18 follows from Eq. 17, while the second equality follows directly from the definition of Eq. 3.

Let us first calculate the zeroth order expansion term of Eq. 14 by setting $\omega = 0$ in the formal expression for the longitudinal spin-susceptibility of Eq. 7 and integrating over the

spatial variables:

$$\chi^{KS}(0) = \int d\vec{r} \int d\vec{r}\,'\chi^{KS}(\vec{r},\vec{r}\,';0) = \int d\vec{r} \int d\vec{r}\,' \sum_{\sigma} \frac{i}{2\pi} \int_{-\infty}^{E_F} dE$$

$$\begin{aligned}
&\big(G^{\sigma}(\vec{r},\vec{r}\,';E)G^{\sigma}(\vec{r}\,',\vec{r};E) - G^{*\sigma}(\vec{r},\vec{r}\,';E)G^{\sigma}(\vec{r}\,',\vec{r};E)\\
&+ G^{\sigma}(\vec{r}\,',\vec{r};E)G^{*\sigma}(\vec{r},\vec{r}\,';E) - G^{*\sigma}(\vec{r}\,',\vec{r};E)G^{*\sigma}(\vec{r},\vec{r}\,';E)\big)\\
&= \int d\vec{r} \sum_{\sigma} \frac{i}{2\pi}\big( - G^{\sigma}(\vec{r},\vec{r};E_F) + G^{*\sigma}(\vec{r},\vec{r};E_F)\big)\\
&= -\int d\vec{r} \sum_{\sigma} \frac{1}{\pi} \operatorname{Im} G^{\sigma}(\vec{r},\vec{r};E_F) = \int d\vec{r} \sum_{\sigma} \rho^{\sigma}(\vec{r},\vec{r};E_F),
\end{aligned} \tag{19}$$

where we made use of Eq. 18 to perform the energy integrations and $\rho^{\sigma}(\vec{r},\vec{r}\ ';E_F) \equiv -1/\pi \operatorname{Im} G^{\sigma}(\vec{r},\vec{r}\,';E_F)$. In order to obtain the result quoted in the main text, one needs to consider the non-magnetic case, *i.e.*, $\rho^{\uparrow}(\vec{r},\vec{r};E) = \rho^{\downarrow}(\vec{r},\vec{r};E) = \rho(\vec{r},\vec{r};E)/2$, thus obtaining

$$\chi^{KS}(0) = \sum_{\sigma} \int d\vec{r}\rho^{\sigma}(\vec{r},\vec{r};E_F) \equiv \rho_F. \tag{20}$$

Next we compute the linear order expansion term $\alpha$, for which we need to calculate the frequency derivative of the spin-susceptibility of Eq. 7,

$$\begin{aligned}
\frac{\partial \chi^0(\vec{r},\vec{r}\,';\omega)}{\partial\omega}\Big|_{\omega=0} &= \frac{i}{2\pi} \sum_{\sigma} \int^{E_F} dE \Big( G^{\sigma}(\vec{r},\vec{r}\,';E) \frac{\partial G^{\sigma}(\vec{r}\,',\vec{r};E+\omega)}{\partial\omega} - G^{*\sigma}(\vec{r},\vec{r}\,';E)\frac{\partial G^{\sigma}(\vec{r}\,',\vec{r};E+\omega)}{\partial\omega}\\
&+ G^{\sigma}(\vec{r}\,',\vec{r};E)\frac{\partial G^{*\sigma}(\vec{r},\vec{r}\,';E-\omega)}{\partial\omega} - G^{*\sigma}(\vec{r}\,',\vec{r};E)\frac{\partial G^{*\sigma}(\vec{r},\vec{r}\,';E-\omega)}{\partial\omega}\Big)\Big|_{\omega=0}\\
&\simeq \frac{i}{2\pi} \sum_{\sigma} \int^{E_F} dE \Big( G^{\sigma}(\vec{r},\vec{r}\,';E) \frac{\partial G^{\sigma}(\vec{r}\,',\vec{r};E)}{\partial E} - G^{*\sigma}(\vec{r},\vec{r}\,';E)\frac{\partial G^{\sigma}(\vec{r}\,',\vec{r};E)}{\partial E}\\
&- G^{\sigma}(\vec{r}\,',\vec{r};E)\frac{\partial G^{*\sigma}(\vec{r},\vec{r}\,';E)}{\partial E} + G^{*\sigma}(\vec{r}\,',\vec{r};E)\frac{\partial G^{*\sigma}(\vec{r},\vec{r}\,';E)}{\partial E}\Big).
\end{aligned} \tag{21}$$

where we made use of Eq. 18 (rightmost expression). We note that one can collect 4 out of the 8 terms in Eq. 21 to form total derivatives of products of two terms:

$$\begin{aligned}
&\sum_{\sigma} G^{*\sigma}(\vec{r},\vec{r}\,';E)\frac{\partial G^{\sigma}(\vec{r}\,',\vec{r};E)}{\partial E} + G^{\sigma}(\vec{r}\,',\vec{r};E)\frac{\partial G^{*\sigma}(\vec{r},\vec{r}\,';E)}{\partial E}\\
&= \sum_{\sigma} \frac{d}{dE}[G^{\sigma}(\vec{r}\,',\vec{r};E)G^{*\sigma}(\vec{r},\vec{r}\,';E)].
\end{aligned} \tag{22}$$

Taking the above into account, the energy integration of these 4 terms can be readily per-

formed, yielding:

$$\frac{\partial\chi^0(\vec{r},\vec{r}\,';\omega)}{\partial\omega}\Big|_{\omega=0} \simeq \sum_\sigma \frac{i}{2\pi}\Big(\int^{E_F} dE\Big(G^\sigma(\vec{r},\vec{r}\,';E)\frac{\partial G^\sigma(\vec{r}\,',\vec{r};E)}{\partial E} + G^{*\sigma}(\vec{r}\,',\vec{r};E)\frac{\partial G^{*\sigma}(\vec{r},\vec{r}\,';E)}{\partial E}\Big) - G^\sigma(\vec{r}\,',\vec{r};E_F)G^{*\sigma}(\vec{r},\vec{r}\,';E_F)\Big). \tag{23}$$

Our goal is to calculate the imaginary part of the above equation. Due to the $i$ factor in front, this requires calculating the real part of the quantities inside the largest parenthesis in the right hand side. The contribution of the terms that have already been energy-integrated is

$$\begin{aligned}&-\operatorname{Re}\Big[\sum_\sigma G^\sigma(\vec{r}\,',\vec{r};E_F)G^{*\sigma}(\vec{r},\vec{r}\,';E_F)\Big] = \\ &-\sum_\sigma\Big(\operatorname{Re}G^\sigma(\vec{r},\vec{r}\,';E_F)\operatorname{Re}G^\sigma(\vec{r}\,',\vec{r};E_F) + \operatorname{Im}G^\sigma(\vec{r},\vec{r}\,';E_F)\operatorname{Im}G^\sigma(\vec{r}\,',\vec{r};E_F)\Big),\end{aligned} \tag{24}$$

while the contribution of the leftover energy integral of Eq. 26 is

$$\begin{aligned}&\operatorname{Re}\Big[\sum_\sigma\int^{E_F} dE\Big(G^\sigma(\vec{r},\vec{r}\,';E)\frac{\partial G^\sigma(\vec{r}\,',\vec{r};E)}{\partial E} + G^{*\sigma}(\vec{r}\,',\vec{r};E)\frac{\partial G^{*\sigma}(\vec{r},\vec{r}\,';E)}{\partial E}\Big)\Big] \\ &= \sum_\sigma\int^{E_F} dE\frac{d}{dE}\Big(\operatorname{Re}G^\sigma(\vec{r},\vec{r}\,';E)\operatorname{Re}G^\sigma(\vec{r}\,',\vec{r};E) - \operatorname{Im}G^\sigma(\vec{r},\vec{r}\,';E)\operatorname{Im}G^\sigma(\vec{r}\,',\vec{r};E)\Big) \\ &= \sum_\sigma\Big(\operatorname{Re}G^\sigma(\vec{r},\vec{r}\,';E_F)\operatorname{Re}G^\sigma(\vec{r}\,',\vec{r};E_F) - \operatorname{Im}G^\sigma(\vec{r},\vec{r}\,';E_F)\operatorname{Im}G^\sigma(\vec{r}\,',\vec{r};E_F)\Big).\end{aligned} \tag{25}$$

Thus, from Eqs. 24 and 25 we finally obtain the expression for the imaginary part of the slope,

$$\begin{aligned}\operatorname{Im}\int d\vec{r}\int d\vec{r}\,'\frac{\partial\chi^0(\vec{r},\vec{r}\,';\omega)}{\partial\omega}\Big|_{\omega=0} &\simeq -\sum_\sigma\int d\vec{r}\int d\vec{r}\,'\frac{1}{2\pi}\operatorname{Im}G^\sigma(\vec{r},\vec{r}\,';E_F)\operatorname{Im}G^\sigma(\vec{r}\,',\vec{r};E_F) \\ &= -\frac{\pi}{2}\sum_\sigma\int d\vec{r}\int d\vec{r}\,'\rho^\sigma(\vec{r},\vec{r}\,';E_F)\rho^\sigma(\vec{r}\,',\vec{r};E_F).\end{aligned} \tag{26}$$

The above equation shows that the linear expansion term of the longitudinal spin-susceptibility is proportional to the product of DOS at the Fermi level of same spin channels, in contrast to the opposite spin channel product appearing in the case of the transverse spin-susceptibility, see Eq. 8 in Ref. 7. In order to obtain the simplified expression quoted in

main text, we adopt the projection of the GFs into angular momentum eigenstates taken in Ref. 7, yielding the following final form for the non-magnetic case,

$$\alpha = -\frac{\pi}{2}\sum_{\sigma}\sum_{L,L'}\rho^{\sigma}_{L,L'}(E_F)\rho^{\sigma}_{L',L}(E_F) \simeq -\frac{\pi}{2}\sum_{\sigma}\sum_{L=d}\rho^{\sigma}_{L,L}(E_F)\rho^{\sigma}_{L,L}(E_F) \sim -\frac{\pi}{4}\rho_F^2, \tag{27}$$

where $L$ and $L'$ are angular momentum labels and we kept only the diagonal term corresponding to the $d$ orbital, which in practice represents virtually all the contribution at the Fermi level. Employing the expression of Eq. 27 into the first order expansion of the susceptibility has been checked to yield good approximate results for energies below 100 meV, see Fig. 2 of the main text.

### A. External static magnetic field

Next we analyze how an external static magnetic field modifies the above results. For this, let us first write down the Dyson equation relating the GFs in absence of a magnetic field (denoted by $G_0(E)$) and in presence of a magnetic field (denoted by $G_B(E)$):

$$G_B(E) = G_0(E) + G_0(E)\cdot\mu_B B\cdot\sigma_z\cdot G_B(E), \tag{28}$$

with $B$ the magnitude of the external magnetic field (we have omitted spatial indexes since they play no role in the derivation). The spinor components of the GFs do not mix and can be separately written as

$$G^{\sigma}_B(E) = \frac{G^{\sigma}_0(E)}{1-\overline{\sigma}\mu_B B G^{\sigma}_0(E)}, \tag{29}$$

with $\overline{\sigma}=1$ ($\overline{\sigma}=-1$) for $\sigma=\uparrow$ ($\sigma=\downarrow$). The imaginary part of the above equation therefore reads

$$\operatorname{Im} G^{\sigma}_B(E) = \frac{\operatorname{Im} G^{\sigma}_0(E)}{\left(1-\overline{\sigma}\mu_B B\operatorname{Re} G^{\sigma}_0(E)\right)^2+\left(\mu_B B\operatorname{Im} G^{\sigma}_0(E)\right)^2} \equiv \xi_{\sigma}(B,E)\operatorname{Im} G^{\sigma}_0(E). \tag{30}$$

Therefore, Eq. 30 shows that the imaginary part of the GFs in presence of the magnetic field is proportional to the imaginary part without the field.

### 1. Non-magnetic case

It is particularly interesting to see how the expansion terms of Eq. 14 are modified by a magnetic field in the non-magnetic case. We begin by the 0th order term of Eq. 19, namely

$$\chi^0(0) = -\frac{1}{\pi}(\operatorname{Im} G_0^{\uparrow}(E_F) + \operatorname{Im} G_0^{\downarrow}(E_F)) = \rho_F, \tag{31}$$

that is, the non-magnetic DOS at the Fermi level. Now inserting Eq. 30 into Eq. 31, we compute how this term is modified by the magnetic field:

$$\begin{aligned}\chi^B(0) &= -\frac{1}{\pi}(\operatorname{Im} G_B^{\uparrow}(E_F) + \operatorname{Im} G_B^{\downarrow}(E_F)) = -\frac{1}{\pi}(\xi_\uparrow(B,E)\operatorname{Im} G_0^{\uparrow}(E_F) + \xi_\downarrow(B,E)\operatorname{Im} G_0^{\downarrow}(E_F)) \\ &= \frac{\xi_\uparrow(B,E)+\xi_\downarrow(B,E)}{2}\rho_F \equiv \xi(B,E)\rho_F,\end{aligned} \tag{32}$$

which is the result quoted in the main text. Note that the scaling factor $\xi(B,E)$ remains unchanged under the reversal of the magnetic moment direction, *i.e.*, $\xi(-B,E) = \xi(B,E)$

The first order expansion term in the non-magnetic case is (see Eq. 26):

$$\alpha_0 = -\frac{1}{\pi}\Big((\operatorname{Im} G_0^{\uparrow}(E_F))^2 + (\operatorname{Im} G_0^{\downarrow}(E_F))^2\Big) = -\frac{\pi}{2}\rho_F^2. \tag{33}$$

Under a magnetic field this is modified as

$$\begin{aligned}\alpha_B &= -\frac{1}{\pi}\Big((\operatorname{Im} G_B^{\uparrow}(E_F))^2 + (\operatorname{Im} G_B^{\downarrow}(E_F))^2\Big) \\ &= -\frac{1}{\pi}\Big(\xi_\uparrow^2(B,E)(\operatorname{Im} G_0^{\uparrow}(E_F))^2 + \xi_\downarrow^2(B,E)(\operatorname{Im} G_0^{\downarrow}(E_F))^2\Big) = -\frac{\pi}{2}\rho_F^2(\xi_\uparrow^2(B,E)+\xi_\downarrow^2(B,E)).\end{aligned} \tag{34}$$

### 2. Low B field expansion of $\xi(B)$

In order to gain insight on the renormalizing term $\xi(B,E)$, we derive its form for low values of the magnetic field. For such purpose we expand the GF in Eq. 29 up to second order in $\mu_B B G_0^\sigma(E)$, *i.e.*,

$$G_B^\sigma(E) \simeq G_0^\sigma(E)\Big(1 + \overline{\sigma}\mu_B B G_0^\sigma(E) + \big(\mu_B B G_0^\sigma(E)\big)^2\Big). \tag{35}$$

After straightforward algebra, the imaginary part of $G_B^\sigma(E)$ can be cast in the following form using the above equation,

$$\operatorname{Im} G_B^\sigma(E) \simeq \operatorname{Im} G_0^\sigma(E)\Big(1 + 2\overline{\sigma}\mu_B B \operatorname{Re} G_0^\sigma(E) + (\mu_B B)^2\big(3(\operatorname{Re} G_0^\sigma(E))^2 - (\operatorname{Im} G_0^\sigma(E))^2\big)\Big). \tag{36}$$

Introducing the above expression into Eq. 32, we obtain the low-field expression for the static susceptibility in the non-magnetic case:

$$\chi^B(0) \simeq \rho_F\Big(1 + (\mu_B B)^2\big(3(\mathrm{Re}\, G_0(E_F))^2 - \frac{\rho_F^2}{4}\big)\Big). \tag{37}$$

One notices that the first order $B$-field expansion term of Eq. 35 has cancelled out, hence the second order one is the lowest contributing term to the renormalization of the Stoner product. Note also that according to the above equation, the renormalization can be $\gtrless 1$ depending on the properties of the electronic structure at the Fermi level.

**References**


[1] N. Papanikolaou, R. Zeller, and P. H. Dederichs, Journal of Physics: Condensed Matter **14**, 2799 (2002).

[2] S. H. Vosko, L. Wilk, and M. Nusair, Canadian Journal of Physics **58**, 1200 (1980).

[3] P. Giannozzi, S. Baroni, N. Bonini, M. Calandra, R. Car, C. Cavazzoni, Davide Ceresoli, G. L. Chiarotti, M. Cococcioni, I. Dabo, et al., Journal of Physics: Condensed Matter **21**, 395502 (2009).

[4] S. Lounis, A. T. Costa, R. B. Muniz, and D. L. Mills, Physical Review Letters **105**, 187205 (2010).

[5] S. Lounis, A. T. Costa, R. B. Muniz, and D. L. Mills, Physical Review B **83**, 035109 (2011).

[6] B. Schweflinghaus, M. dos Santos Dias, A. T. Costa, and S. Lounis, Phys. Rev. B **89**, 235439 (2014).

[7] S. Lounis, M. dos Santos Dias, and B. Schweflinghaus, Phys. Rev. B **91**, 104420 (2015).

[8] J. F. Janak, Physical Review B **16**, 255 (1977).

[9] B. Lazarovits, L. Szunyogh, and P. Weinberger, Phys. Rev. B **65**, 104441 (2002).

[10] H. Beckmann and G. Bergmann, Physical Review B **55**, 14350 (1997).

[11] K. Wildberger, P. Lang, R. Zeller, and P. H. Dederichs, Phys. Rev. B **52**, 11502 (1995).
